# Supplementary material for: The Benefit of Sex in Noisy Evolutionary Search
Source: arXiv:1502.02793 source file (2015-02-10)
Supplement: Supplementary file 1 [file appendix.tex]

The following theorem was stated as Theorem~\ref{??}; here we restate the theorem, along with a proof.
